# Supplementary material for: ConDor: Self-Supervised Canonicalization of 3D Pose for Partial Shapes
Source: arXiv:2201.07788 source file (2022-04-14)
Supplement: Supplementary file 1 [file 01_supp.tex]

\begin{Lemma}
A map $t: \mathcal{X} \rightarrow g$ satisfying the equivariance property:
 $t(g.x) = t(x)g^{-1}$ for all $x \in \mathcal{X}$ and $g \in G$ induces a canonicalizing map $s: \mathcal{X} / \sim \rightarrow \mathcal{X}$ defined by $s(\overline{x}) := t(x).x$ where $\overline{x} \in \mathcal{X} / G := \mathcal{X} / \sim$ is the equivalence class (or orbit) of $x$. Please see the supplementary material for a proof.
 \label{lemma:can_transform}
\end{Lemma}
\begin{proof}
By construction $t(x).x \in \overline{x}$ we simply have to verify that $t(x).x$ is invariant by the action of $G$. We have $t(g.x).(g.x) = t(x)g^{-1}(g.x) = t(x).x$. \Srinath{could go to appendix}
\end{proof}

\Adrien{technically this is false, this is true up to xyz -> yzx change of coordinate but is seems that this technical point would complicate the discussion and this is actually just a convention}

the tensors $\Tilde{H}^{\ell}(X)$ are rotation invariant as:
\[
\begin{aligned}
\Tilde{H}^{\ell}_{ijk}(R.X)
&
= 
\langle Z^{\ell}_{i,:,j}(R.X), \Tilde{f}^{\ell}_{:,j,k}(R.X)\rangle
\\
&
=
\langle D^{\ell}(R)Z^{\ell}_{i,:,j}(X), D^{\ell}(R) \Tilde{f}^{\ell}_{:,j,k}(X)\rangle
\\
&
=
\langle Z^{\ell}_{i,:,j}(X),  \Tilde{f}^{\ell}_{:,j,k}(X)\rangle
=
\Tilde{H}^{\ell}_{ijk}(X)
\end{aligned}
\]
\Rahul{Can defer the readers to supplementary for showing that the dot product is rotation invariant?}

\begin{table}[ht]
\begin{center}
\scalebox{0.84}{
\begin{tabular}{|c|c|c|c|}
\hline
  & \multicolumn{2}{|l|}{full} \\
  \hline
  Methods & $\{I\}$ & $\mathrm{SO}(3)$  \\
  \hline
  PCA+Pointnet & 0.7731 & 0.6490  \\
%   PointNet \cite{} & & & &\\
%   PointNet++ \cite{} & & & &\\
%   Point2Seq \cite{} & & & &\\
%   SphericalCNN \cite{} & & & &\\
%   LDGCNN \cite{} & & & &\\
%   SO-Net \cite{} & & & &\\
%   PRIN \cite{} & & & &\\
%   CaCa \cite{} & & & &\\
  CaCa+PointNet & 0.7680 & 0.7248 \\
  Compass+PointNet & 0.8051 & 0.7220  \\
  Ours+PointNet & 0.7618 & 0.7458 \\
%   Ours+DGCNN & & & &\\
  \hline
\end{tabular}}
\caption{Classification accuracy on the ModelNet40 dataset when training without augmentation. The $\{I\}$ column reports the accuracy attained when testing on the cloud in the canonical orientation provided
by the dataset and the $\mathrm{SO}(3)$ column when testing under arbitrary rotations. Best result for each row in bold. In this table we only include accuracy with respect to other canonicalization methods for comparison and do not include the state-of-the-art that performs better than all the methods listed in the table.
\label{table:ModelNet40}}
\end{center}
\end{table}

% \subsection {Partial shape canonicalization}
\begin{table}[]
\centering
\scalebox{0.9}{
\begin{tabular}{|cc|}
\hline
\multicolumn{2}{|c|}{\textbf{L2 Norm}}                               \\ \hline
\multicolumn{1}{|c|}{Avg. Single Category} & Multi Category \\ \hline
\multicolumn{1}{|c|}{0.0291}               & 0.0326         \\ \hline
\end{tabular}
}
\caption{\textbf{Translation error:} L2 Norm of the translation vector categories.\label{table:translation}}
\end{table}

\parahead{Performance on full shape canonicalization with partiality and translation}
We evaluate the canonicalization of full shapes using our network trained on full and partial shapes. From table \ref{table:canonicalization_metrics} we observe that on average both our models \textbf{Ours(F)} and \textbf{Ours(F+P)} perform the same on the canonicalization metrics for full shapes. For a few categories such as \textit{lamp, car, chair, watercraft}, introducing partial shapes in the training improves its performance on the canonicalization metrics. Whereas introducing occlusion during training degrades the performance for category $bench$.

\Srinath{Experiment request: what happens if we re-train the same network multiple times with different random seeds? Do we get different canonical frames?}

\Srinath{Application Idea: We can actually canonicalize meshes right? We can sample points on a mesh, canonicalize it, get the rotation/translation and apply it to the original mesh. Should we show some examples of this? We could also show this for partial meshes. This would be very cool}

\parahead{3D Registration}
%
\iffalse
Our second indirect canonicalization evaluation is to compute the registration error following \cite{deepgmr}.
Given two (full) shapes of the same instance that need to be registered, we compute an equivariant frame for both shapes, then align the two frames before computing the root mean square error (RMSE) between corresponding points.
We compare our RMSE, Ours(F)(0.4961), Ours(F+P)(0.0331) with Deep Closest Points~\cite{wang2019deep} (0.131), Deep GMR~\cite{deepgmr} (0.077), CaCa (\textbf{0.070}), Compass (0.4866) and PCA (0.7148).
We note that our method does not perform well in this task as we predict a frame $E \in O(3)$ which can have reflection symmetries, we observed many such symmetries like left-right reflection for planes. However registration works well w.r.t. to Chamfer Distance metric which is symmetry agnostic as suggested by the scores Ours(F) (0.0396), Ours(F+P) (\textbf{0.0331}) CaCa (0.0395). We also note that Ours(F+P) noticeably decrease RMSE compared to  Ours(F) as during training frame consistency is enforced between the full shape and a randomly rotated partial by the $\mathcal{L}_{rest}$ loss of \cref{eq:frame_restriction_loss}.
\fi

% \Srinath{For classification, two things: infer on modelnet and then classify. Classification on partial shapes.}
\Rahul{It might be good to give the readers a sense of inter-canonicalization metrics, for instance if one model performs better in con but worse in eq and another model performs bad in eq but good in con, which model is the better one? I think it might be good to give some intuition/insight into that too.}

\Srinath{Compare runtimes}
% \Srinath{What happens if we do not have the segmetnation part. Does performance degrade?} \Rahul{Removing segmentation doesnt change anything}

\input{content/text/tables/ablation_degree_partiality}

\todo{co-canonicalization }

\section{Keypoint Transfer}
More specifically, we transfer the keypoint annotation by computing the directional vector in the source point cloud and use the corresponding capsule in the same direction in the target point cloud to find its nearest neighbor.

\begin{Lemma}
A map $t: \mathcal{X} \rightarrow g$ satisfying the equivariance property:
 $t(g.x) = t(x)g^{-1}$ for all $x \in \mathcal{X}$ and $g \in G$ induces a canonicalizing map $s: \mathcal{X} / \sim \rightarrow \mathcal{X}$ defined by $s(\overline{x}) := t(x).x$ where $\overline{x} \in \mathcal{X} / G := \mathcal{X} / \sim$ is the equivalence class (or orbit) of $x$. Please see the supplementary material for a proof.
 \label{lemma:can_transform}
\end{Lemma}
\begin{proof}
By construction $t(x).x \in \overline{x}$ we simply have to verify that $t(x).x$ is invariant by the action of $G$. We have $t(g.x).(g.x) = t(x)g^{-1}(g.x) = t(x).x$. 
\end{proof}
\Rahul{Do we need this? Need to fix the box}
