# Supplementary material for: ConDor: Self-Supervised Canonicalization of 3D Pose for Partial Shapes
Source: arXiv:2201.07788 source file (2022-04-14)
Supplement: Supplementary file 2 [file rmse_metrics.tex]

\begin{table}[ht]
\begin{center}
\scalebox{0.84}{
\begin{tabular}{|c|c|c|c|c|}
\hline
  & \multicolumn{2}{|l|}{RMSE} & \multicolumn{2}{|l|}{Chamfer}\\
  \hline
  Methods & avg & multi  & avg & multi\\
  \hline
  \multicolumn{5}{|c|}{IC} \\
  \hline
  PCA & & 0.7148 & &\\
  CaCa \cite{sun2020canonical} & 0.3993 & 0.1529 &  & \\
  Compass \cite{spezialetti2020learning} &  & 0.4866 & &\\
  Ours (F) & & 0.4961 & & \\
  Ours (F+P) & & 0.4044 & & \\
\hline
  \multicolumn{5}{|c|}{GC} \\
  \hline
  PCA & & 0.4741 & &\\
  CaCa \cite{sun2020canonical} & 0.3638 & 0.6675 & &\\
  Compass \cite{spezialetti2020learning} &  & 0.7193 & &\\
  Ours (F) & & 0.6588 & & \\
  Ours (F+P) & & 0.6625 & & \\
  \hline
\end{tabular}}
\caption{}
\end{center}
\end{table}
\Rahul{Not sure how CC makes sense for RMSE as we don't have correspondence between different shapes}
